# Supplementary material for: A Reinforcement Learning Environment for Directed Quantum Circuit Synthesis
Source: arXiv:2401.07054 source file (2024-01-13)
Supplement: Supplementary file 1 [file X_appendix.tex]

% \cleardoublepage
% \section*{\uppercase{Appendix}}

% \subsection*{Optimizing the learning rate }\label{subsec: optlearningrate}
% Representing one of the most essential parameters of gradient-based ML algorithms, we preliminary investigate the influence of the learning rate $\alpha$ on the agents' performance, corresponding to the reached reconstruction circuit-depth $\Lambda$. To get an overview of the dependency between the final quality of the trained agents and $\alpha$, we tested a variety of learning rate values. (0.00001, 0.0001, 0.0003, 0.0005, 0.0007, 0.001, 0.01) We chose this specific selection of values since it contains the default learning rates for both tested algorithms PPO ($\alpha$ = 0.0003) and A2C ($\alpha$ = 0.0005) and an additional variation around these values. On the basis of intuition gained through experiments carried out during the development of the RL environment, we defined the $SFE$ value to be 0.001. As a reward technique, we used the 'bare-step-penalty' implementation of the RL environment given in equation \ref{eq: reward2}, representing the sparser reward technique of the available options. The baselines in the plots obey the standard parameters for the number of qubits, circuit-depth and $SFE$. Since during the random sampling no training process is involved, the definition of the learning rate is irrelevant.\indent 
% We defined the criterion for the best learning rate within the tried selection of values to be the $\alpha$-value producing the lowest final reconstruction circuit-depth $\Lambda$ in a trained agent.

% \subsubsection*{PPO}
% \begin{figure}[htbp]
%     \centering
%     \includegraphics[width=\linewidth,keepaspectratio]{images/PPO_Learning_rateFinesse_plot.png}
%     \caption{ Proceeding of the reconstruction circuit-depth $\Lambda$ of a variety of PPO-agents together with the first standard deviation plotted against the number of steps during training. The agents were trained on the 2-qubit DQCS problem of circuit-depth $\lambda = 5$ using different learning rates respectively, while all other parameters are maintained constant.} 
%     \label{fig: adjustlearningrate}
% \end{figure}
% Figure \ref{fig: adjustlearningrate} shows the training runs of PPO-agents varying in their learning rates $\alpha$ keeping all other parameters at the defined standard values given above. It gets apparent, that the best performance is achieved using a learning rate $\alpha = 0.001$, showing the lowest reconstruction circuit-depth $\Lambda$ at the end of the training. A reconstruction circuit-depth $\Lambda = 100\%$ can be interpreted as a recreation of every target by the agent, utilizing a circuit equivalent to the one used at initialization. Hence the reached absolute reconstruction circuit-depth of approximately $\Lambda = 115\%$ indicates a high target-finding probability. Further, the slope at the end of the training curve of $\alpha = 0.001$ is < 0, adverting a still ongoing learning process of the agent, possibly leading to an even smaller $\Lambda$ if trained longer. Observing the standard deviation of the $\alpha = 0.001$ curve, the difference to the random baseline becomes evident, ensuring the performance of the respective agents. Due to the mentioned reasons, we set $\alpha = 0.001$ to be the standard learning rate for all upcoming PPO experiments. However, this decision just arose by analyzing a fairly small variety of different $\alpha$-values, implying that further optimization of $\alpha$ is indeed possible and meaningful.\indent
% Analyzing further, for $\alpha$-values below 0.001 a direct dependence between the absolute value of $\alpha$ and the observed learning performance holds. Put differently, the lower the $\alpha$-value, the slower and weaker the learning process. This is also intuitively reasonable imagining the slower update movement on the weight hyperplane of the neural network represented by the agent. The examined $\alpha$-value above 0.001, $\alpha = 0.01$, shows no learning behavior at all, indicating that the step size is too big to create a trainable agent. An explanation for this behavior might include the skipping of minima in the weight hyperplane by big update steps induced through the large $\alpha$-value. \newline

% \subsubsection*{A2C}
% Figure \ref{fig: A2Cadjustlearningrate} shows the training runs of A2C-agents varying in their learning rates $\alpha$ keeping all other parameters at the standard setting given above. Overall, the graph shows a weak performance of the A2C-algorithm on the DQCS problem when compared to the PPO approach, not reaching reconstruction circuit-depths $\Lambda$ below $195\%$ regardless of which learning rate is applied. The variation of learning rate seems to have no big influence on the behavior of the agent, although the agents using smaller $\alpha$-values tend to achieve a lower $\Lambda$ in general. The learning procedure mostly occurs in a step-wise manner, forming planes in which almost no improvement takes place over large periods of training. In general, it can be stated that the curves of $\alpha = 0.0005$, $\alpha = 0.0003$ and $\alpha = 0.00001$ show the best results regarding the final reconstruction circuit-depth $\Lambda$. A critical point regarding the behavior of A2C involves the fact that all of the tried approaches show an overlap of the first standard deviations with the random baseline. This emphasizes the insufficient performance of the A2C-algorithm on the task.\indent
% Since we found the PPO-approach to be more competitive than the A2C-algorithm during the learning rate optimization, PPO is the algorithm of choice for all following experiments. 
% \begin{figure}[htbp]
%     \centering
%     \includegraphics[width=\linewidth,keepaspectratio]{images/A2C_Learningrate_Finesse_plot.png}
%     \caption{Proceeding of the reconstruction circuit-depth $\Lambda$ of a variety of A2C-agents together with the first standard deviation plotted against the number of steps during training. The agents were trained on the 2-qubit DQCS problem of circuit-depth $\lambda = 5$ using different learning rates respectively, while all other parameters were maintained constant.} 
%     \label{fig: A2Cadjustlearningrate}
% \end{figure}


% \subsection*{Optimizing the Standard Fidelity Error (\textit{SFE})}
% A hyperparameter introduced to simplify the generation of the defined target state by reducing the accepted fidelity to a value $<1$ represents the standard fidelity error ($SFE$) (see equation \ref{eq: reward2}). In the following, we trained PPO-agents utilizing the standard environment setting introduced in section \ref{subsec: optlearningrate} including the optimized learning rates obtained in the same section, together with a selection of different $SFE$-values. (0, 0.001, 0.01, 0.1, 0.2 and 0.3) We chose this specific value selection to cover an area enabling only solutions close to the actual target, disregarding large $SFE$-values > 0.3. We set up the random baseline using the standard parameters, involving $SFE = 0.001$ and a learning rate of 0.001. \newline
% As depicted by the graph in figure \ref{fig: PPO-sfe}, all curves apart from $SFE$ = 0 show an improvement in performance when compared to the random baseline, exceeding the first standard deviation. Further, it gets apparent that the approach using $SFE = 0$ creates a poor performance not falling under a reconstruction circuit-depth $\Lambda$ of 180\%. This possibly originates from its restriction to the preparation of the exact target state, hampered by rounding errors. Hence, a slight increase in $SFE$ drastically decreases $\Lambda$ to approximately 110\%, leading to a cluster of curves including '$SFE = 0.001$', '$SFE = 0.01$' and '$SFE = 0.1$' showing only minor variations between each other. The curve of $SFE = 0.001$ proceeds exactly like the curve of  $SFE = 0.01$ and is thus hidden underneath. By further increasing the $SFE$, $\Lambda$ can be decreased even more, resulting in a final reconstruction circuit-depth of roughly 70\% as exhibited by the curves of $SFE = 0.2$ and $SFE = 0.3$. Reconstruction circuit-depths far below 100\% indicate the generation of states slightly different from the actual defined target. The acceptance of such solutions is possible due to the enlarged solution-space created by higher $SFE$-values. This hints the preparation of states which are unequal but related to the actual target. Although indicating an inaccurate solution this circumstance can be indeed useful if only approximate target structures or targets obeying a certain characteristic are searched.\newline
% \begin{figure}[htbp]
%     \centering
%     \includegraphics[width=\linewidth,keepaspectratio]{images/PPO_SFE_Finesse_plot.png}
%     \caption{ Proceeding of the reconstruction circuit-depth $\Lambda$ of a variety of PPO-agents plotted against the number of steps during training, together with the first standard deviation. The agents were trained on the 2-qubit DQCS problem of circuit-depth $\lambda = 5$ using different $SFE$-values respectively, while all other parameters including the learning rate are maintained constant.} 
%     \label{fig: PPO-sfe}
% \end{figure} 

% In general, the dependency of the reconstructed circuit-depth $\Lambda$ on the $SFE$ is intuitively understandable. By increasing the $SFE$ the space of accepted states, which are interpreted as equivalent to the actual target, grows. Thus the number of target-preparing circuits rises, enhancing the probability of a valid circuit creation. This in turn decreases the average reconstructed circuit-depth $\Lambda$. Hence the decision about the optimal $SFE$ is governed by a trade-off between performance and the closeness of the generated solutions to the actual target states. Properly weighing this trade-off, we selected $SFE = 0.001$ to be the standard value for the upcoming experiments, producing a comparatively competitive reconstruction circuit-depth $\Lambda$, while maintaining a narrow space of valid solutions. 
